# Supplementary material for: MD2G-Cast: Relay-Coordinated Multicast for Scalable Volumetric Streaming over MoQ
Source: arXiv:2608.10020 source file (2026-08-09)
Supplement: Supplementary file 1 [file SectionA.tex]

\section{System Inputs and Workload Profiling}
\label{sec:appendix_inputs}

This supplement summarizes the workload inputs used by the MD2G-Cast controller, including heterogeneous bandwidth traces and time-varying FoV-overlap statistics.

\subsection{Network Bandwidth Traces}
We use heterogeneous access traces spanning 4G, 5G, Wi-Fi, and fiber-optic settings. Figure~\ref{fig:bw_cdf} shows the raw trace distributions before Mininet applies the type-specific access-link caps used during the experiments. The distributions are broadly separated: 4G and Wi-Fi exhibit heavier low-bandwidth tails, whereas 5G and fiber traces are generally right-shifted and contain higher throughput samples. This diversity provides varied operating conditions for evaluating adaptive Base/Enhanced delivery under heterogeneous access.

\subsection{FoV-Overlap Dynamics}
We derive FoV-overlap statistics over time from the head-motion traces used in the evaluation.
Figure~\ref{fig:fov_overlap} reports the temporal evolution of the mean overlap together with the interquartile range. The overlap changes over time, providing the relay with a time-varying signal that can be used when revisiting group assignments. The figure is descriptive and does not by itself establish a performance advantage over static grouping.

\begin{figure}[t]
    \centering
    \includegraphics[width=0.8\linewidth]{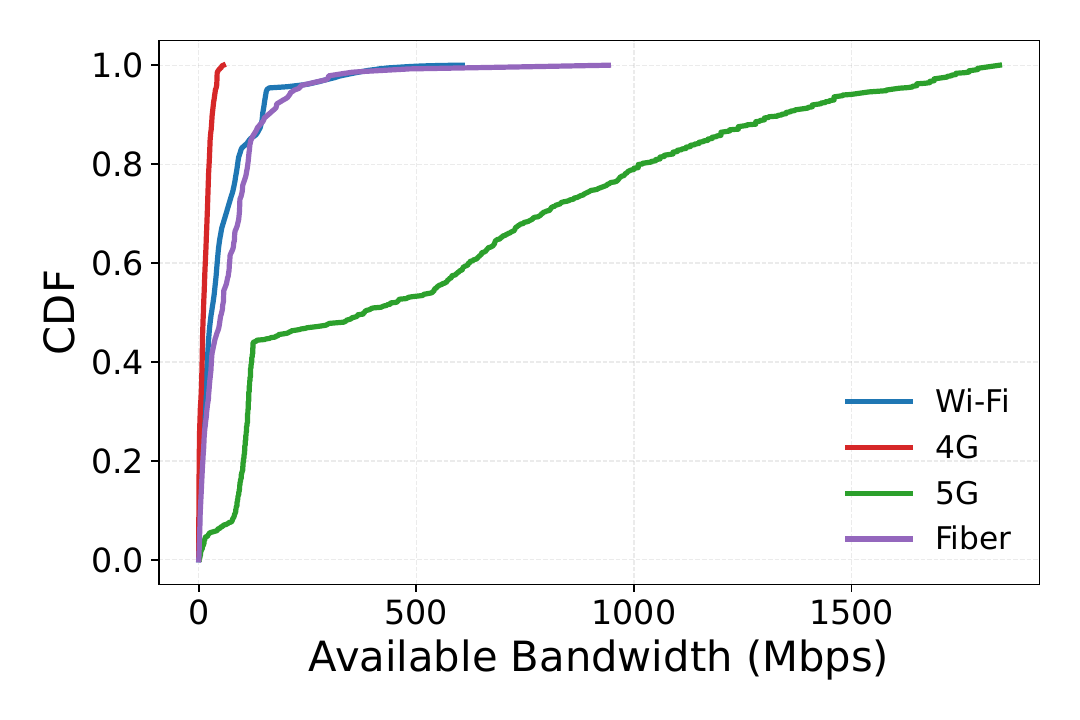}
    \caption{Raw bandwidth trace distributions before access-link caps are applied.}
    \Description{Empirical bandwidth distributions for Wi-Fi, 4G, 5G, and fiber traces before experimental access-link caps are applied.}
    \label{fig:bw_cdf}
    \vspace{-1em}
\end{figure}

\begin{figure}[t]
    \centering
    \includegraphics[width=0.8\linewidth]{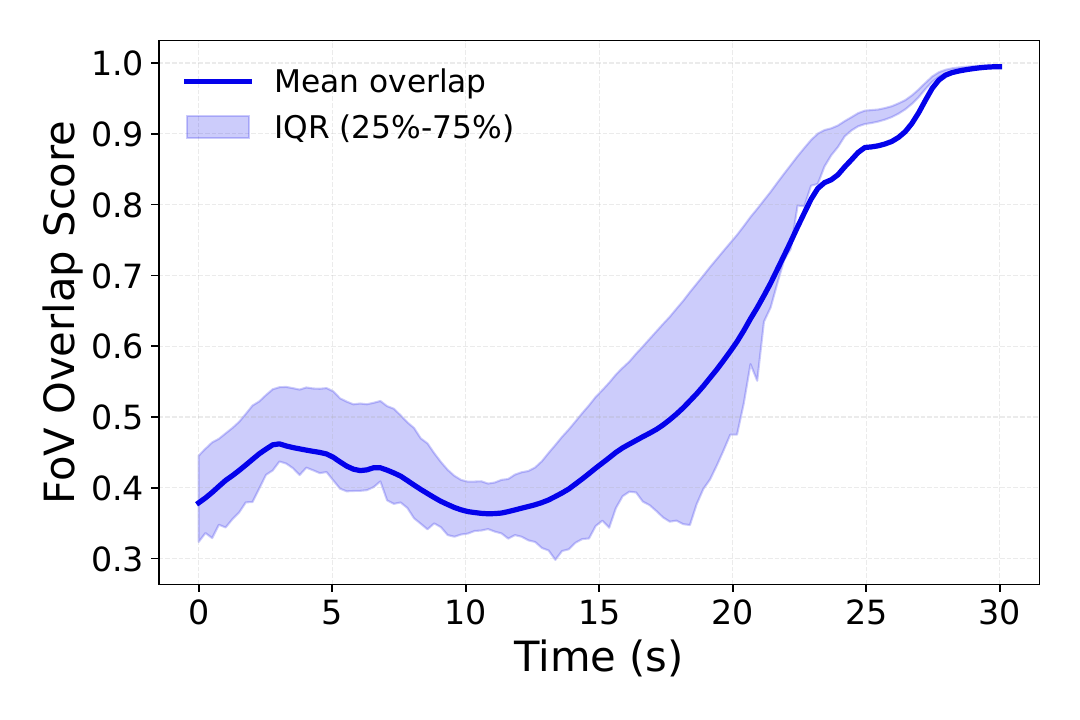}
    \caption{Representative 30\,s window of FoV overlap across users.}
    \Description{Mean and interquartile range of FoV overlap during a representative 30-second head-motion window.}
    \label{fig:fov_overlap}
    \vspace{-1em}
\end{figure}
