# Supplementary material for: MD2G-Cast: Relay-Coordinated Multicast for Scalable Volumetric Streaming over MoQ
Source: arXiv:2608.10020 source file (2026-08-09)
Supplement: Supplementary file 2 [file SectionB.tex]

\section{Policy Architecture, Objective, and Training Details}
\label{sec:appendix_policy}

This appendix provides implementation details of the PPO-based control policy, the teacher--student distillation setup, and the runtime parameters used in MD2G-Cast.

\subsection{Deployment Locus and Model Architecture}
To satisfy real-time control constraints at relays, MD2G-Cast separates offline supervision from online inference.
The high-capacity Teacher-512 model is used only during training, while the lightweight Student-128 model is deployed in the relay-side control loop during runtime.

As summarized in Table~\ref{tab:model_arch}, policy inference in MD2G-Cast is executed at relay-side controllers, and clients follow the relay-issued decisions through the control path. For comparison, Rolling retains client-local adaptation and independent delivery. It therefore serves as an independent delivery reference rather than a same-substrate MoQ baseline. The controlled MoQ comparison is provided by Heuristic and Clustering, which share the delivery substrate used by MD2G-Cast.


\begin{table}[t]
\centering
\caption{Model architectures and deployment loci.}
\label{tab:model_arch}
\begin{tabularx}{\columnwidth}{@{}l >{\raggedright\arraybackslash}X >{\raggedright\arraybackslash}X@{}}
\toprule
\textbf{Component} & \textbf{Network Architecture} & \textbf{Decision Locus} \\ \midrule
MD2G Teacher (Offline) & 3-layer MLP with 512 hidden units & Training only \\
MD2G Student (Online) & 2-layer MLP with 128 hidden units & Relay-side controller \\
Rolling Baseline & Client-local adaptive controller & Client \\
\bottomrule
\end{tabularx}
\vspace{-1em}
\end{table}

\subsection{Training Objective and Runtime Hyperparameters}
The MD2G-Cast system utility is defined as
\begin{equation}
U_i=
\operatorname{clip}_{[0,1]}
\left(
0.25R_{o,i}+0.60R_{q,i}-0.15R_{b,i}
\right).
\end{equation}
Clipping is applied to each sample or accounting window before the expected-client aggregation.

Here, \(R_q\) combines the point-set configuration available at the receiver with delivery-interval and stall penalties. \(R_o\) measures grouping efficiency, and \(R_b\) penalizes bandwidth inefficiency. Table~\ref{tab:runtime_hyperparameters} summarizes the main optimization and runtime parameters used in the experiments.

\begin{table}[t]
\centering
\caption{Policy and system runtime hyperparameters.}
\label{tab:runtime_hyperparameters}
\begin{tabular}{@{}ll@{}}
\toprule
\textbf{Parameter} & \textbf{Value} \\ \midrule
\multicolumn{2}{@{}l}{\textit{Policy Optimization and Distillation}} \\
Actor learning rate & $3 \times 10^{-5}$ \\
Critic learning rate & $1 \times 10^{-4}$ \\
PPO clip range \(\epsilon\) & 0.2 \\
Distillation coefficient & 0.1 \\
\midrule
\multicolumn{2}{@{}l}{\textit{Runtime Control}} \\
Controller update interval & 1.0\,s \\
Runtime FoV-overlap threshold & 0.5 \\
Bandwidth EMA update & \(B_u \leftarrow 0.3 B_u + 0.7 B_u^{\text{inst}}\) \\
Hysteresis count (enable / disable) & 1 / 2 \\
Quality-history window length & 15 \\
\bottomrule
\end{tabular}
\vspace{-1em}
\end{table}
