# Supplementary material for: MD2G-Cast: Relay-Coordinated Multicast for Scalable Volumetric Streaming over MoQ
Source: arXiv:2608.10020 source file (2026-08-09)
Supplement: Supplementary file 3 [file SectionC.tex]

\section{Measurement Methodology and Experimental Controls}
\label{sec:appendix_methodology}

This appendix defines the measurement methodology, aggregation rules, and experimental controls used in our evaluation. The goal is to separate common measurement procedures from the strategy-specific mechanisms under comparison.
\subsection{Metric Definitions and Aggregation}
\label{sec:appendix_metrics}

\paragraph{Steady-state delivery interval.}
We measure the receiver-side inter-arrival interval between useful media payloads and smooth it using the same exponential moving average for every strategy. The reported value is bounded to $[1,500]$\,ms under the shared fallback and reporting rules. This metric characterizes sustained delivery continuity; it is neither network RTT nor end-to-end capture-to-render latency.

\paragraph{Throughput and bandwidth utilization.}
We estimate instantaneous throughput from passive receive-path counters using cumulative received bytes and elapsed wall-clock time, then convert the result to Mbps. Unless a figure caption states otherwise, throughput refers to achieved client-side receive throughput under the full protocol stack and workload rather than to configured link capacity.

\paragraph{Stall behavior.}
A stall interval is declared when the playout-buffer model indicates insufficient backlog or when the delivery interval exceeds the configured threshold, with both conditions evaluated on the same control cadence. We record both stall duration in seconds and stall event counts. For \(R_q\), the normalized stall penalty is derived from cumulative stall duration through a saturating mapping with a fixed time constant.

\paragraph{Quality and system utility.} We distinguish delivered quality from the final system objective. The quality term $R_q$ combines the point-set configuration available at the receiver with normalized delivery-interval and stall penalties and is bounded to $[0,1]$. The grouping term $R_o$ measures the efficiency of shared delivery, while $R_b$ captures bandwidth inefficiency. These terms form the system utility defined in Section~\ref{sec:appendix_policy}. This distinction allows the evaluation to separate delivered quality from the broader trade-off among sharing, continuity, and network cost.


\paragraph{Aggregation.} All primary measurements exclude the first 30\,s of each 120\,s run. System utility is clipped at the sample or accounting-window level before averaging over the expected client population. An expected client without a valid served sample contributes zero. Delivery interval percentiles follow the convention stated by the corresponding figure. All compared strategies use the same warm-up and aggregation procedure for shared metrics.

\paragraph{Control cadence.} The adaptation loop advances at the same one-second interval for every strategy. Shared measurements use common sampling, normalization, and bounded post-processing rules.

\subsection{Testbed and Topology Configuration}
\label{sec:appendix_testbed}

Table~\ref{tab:testbed} summarizes the emulated topology and its key configuration parameters. The deployment follows a hierarchical relay tree in which a publisher feeds a root relay, leaf relays serve end clients, and access links are driven by traces subject to configured caps. User population scales from 10 to 100 concurrent clients, and every strategy follows the same run duration and measurement procedure unless explicitly stated otherwise.

\begin{table*}[t]
\centering
\small
\caption{Experimental configuration used throughout the evaluation.}
\label{tab:testbed}
\begin{tabular}{@{}p{0.22\linewidth}p{0.72\linewidth}@{}}
\toprule
\textbf{Item} & \textbf{Setting} \\
\midrule
Topology & One publisher, one root relay, two leaf relays, and up to 100 clients distributed across two access subnets. \\
Core links & The publisher to root link provides 1\,Gbps capacity with 1\,ms propagation delay. Root to leaf links are provisioned according to the evaluated user scale with 5\,ms propagation delay. \\
Access profiles & Trace driven Wi-Fi, 4G, 5G, and fiber access. Link rates follow the corresponding traces subject to the experimental access caps. \\
Mixed access & The heterogeneous configurations combine Wi-Fi, 4G, 5G, and fiber users using the default-mix, Wi-Fi-dominant, and 5G-dominant population profiles. \\
User scale & $N\in\{10,20,40,60,100\}$. \\
Run duration & 120\,s with a 30\,s warm-up. \\
Control interval & 1.0\,s. \\
Media workload & The \textit{Red and Black} sequence partitioned into complementary Base and Enhanced point sets and encoded as separate V-PCC atlas streams. \\
Source partition & Fixed Base ratio $\rho=0.6$ with deterministic index-stride sampling; the remaining points form the Enhanced complement. \\
Execution platform & 32-vCPU Ubuntu server with 160\,GB RAM. \\
\bottomrule
\end{tabular}
\vspace{-1em}
\end{table*}

\subsection{Controlled Variables and Intended Experimental Differences}
\label{sec:appendix_variables}

We separate the experimental factors held constant across strategies from the mechanism differences intentionally preserved for comparison.

\paragraph{Controlled variables.} Across all compared strategies, we use the same content workload, user population for each scenario, network-trace pools, topology family, access-link constraints, experiment duration, warm-up interval, and measurement methodology. Shared metrics, including delivery interval, throughput, stall-related quantities, Enhanced exposure, and system utility, follow the same definitions and aggregation rules wherever they are applicable to the corresponding delivery mechanism.

\paragraph{Intended experimental differences.} The evaluation deliberately preserves the behaviors that define each strategy. MD2G-Cast, Heuristic, and Clustering operate over the same MoQ-based delivery substrate but differ in how users are grouped and how optional Enhanced delivery is admitted. Rolling serves as an independent-delivery reference with client-local adaptation and therefore retains its native delivery and adaptation behavior. These differences are part of the evaluated mechanisms rather than uncontrolled experimental variation.

This separation provides a controlled basis for comparison. Same-substrate comparisons isolate the effect of relay-side grouping and admission decisions, while the Rolling comparison characterizes the broader system-level difference between coordinated multicast delivery and independent per-client delivery. All reported metrics are computed under the common measurement definitions described above, while strategy-specific transport and control behavior is preserved by design.
