# Supplementary material for: MD2G-Cast: Relay-Coordinated Multicast for Scalable Volumetric Streaming over MoQ
Source: arXiv:2608.10020 source file (2026-08-09)
Supplement: Supplementary file 4 [file SectionD.tex]

\section{Teacher and Student Distillation Fidelity}
\label{sec:appendix_distillation}

Student-128 is trained with teacher guidance on its Enhanced-admission branch. We evaluate whether the compact controller preserves similar system-level outcomes under the Wi-Fi setting with 100 users.

\begin{figure}[t]
\centering
\includegraphics[width=0.90\linewidth]{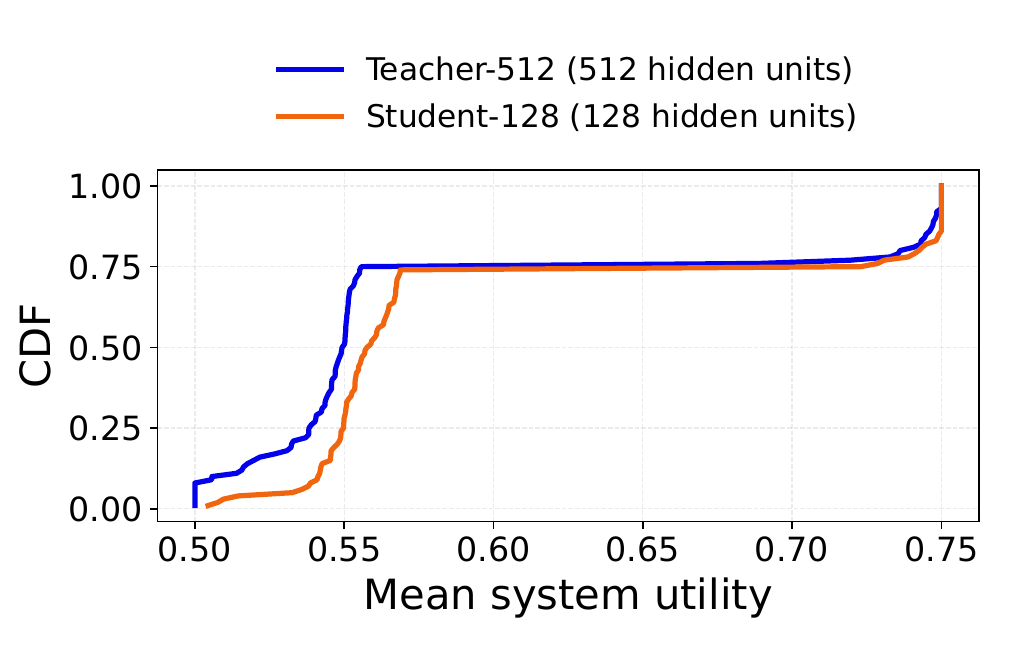}
\caption{System utility distributions for Teacher-512 and Student-128 with 100 Wi-Fi users.}
\Description{Empirical cumulative distributions of per-client mean system utility for the Teacher-512 and Student-128 policies under the Wi-Fi 100-user workload.}
\label{fig:distillation}
\vspace{-2em}
\end{figure}

Figure~\ref{fig:distillation} reports the empirical distribution of per-client mean system utility. The Student-128 distribution closely follows the Teacher-512 distribution across most of the observed range. Together with the inference profile in the main paper, this result shows that the compact model retains similar system utility in the evaluated setting while substantially reducing model size and inference cost.
