# Supplementary material for: MD2G-Cast: Relay-Coordinated Multicast for Scalable Volumetric Streaming over MoQ
Source: arXiv:2608.10020 source file (2026-08-09)
Supplement: Supplementary file 5 [file SectionE.tex]

\section{Artifact and Reproducibility Details}
\label{sec:artifact_reproducibility}

\subsection{Public Artifact and Lightweight Inputs}

The public artifact provides the implementation, Mininet orchestration scripts, trace manifests, and analysis code. Because the full media assets exceed the supplementary upload limit, the packaged Base and Enhanced clips are shortened 10-second inputs intended only for end-to-end pipeline validation. They are not used to produce the measurements reported in the paper. All reported experiments use the full 120-second Base and Enhanced workloads described above.
