# Supplementary material for: MD2G-Cast: Relay-Coordinated Multicast for Scalable Volumetric Streaming over MoQ
Source: arXiv:2608.10020 source file (2026-08-09)
Supplement: Supplementary file 6 [file Section_Ablation.tex]

\section{Matched Relay-Control Ablation}
\label{sec:appendix_ablation}

We evaluate four relay-control variants under the default heterogeneous mix with 60 users. All variants use the same workload, traces, topology, 120\,s run duration, 30\,s warm-up, and measurement procedure, and differ only in the relay-control decision rule. System utility follows the same definition as the main paper. The reported values summarize three matched trials.

\begin{table}[t]
\centering
\caption{Component summary of the matched relay-control ablation.}
\label{tab:ablation_components}
\small
\setlength{\tabcolsep}{4pt}
\begin{tabular}{@{}lccc@{}}
\toprule
\textbf{Variant} & \textbf{Utility} & $R_q$ & $R_b$ \\
\midrule
Full MD2G-Cast & $0.716\pm0.004$ & 0.777 & 0.005 \\
Fixed grouping & $0.712\pm0.003$ & 0.770 & 0.002 \\
Random feasible action & $0.703\pm0.014$ & 0.773 & 0.075 \\
Rule-only controller & $0.718\pm0.006$ & 0.782 & 0.007 \\
\bottomrule
\end{tabular}
\vspace{-2em}
\end{table}

The mean grouping term is 1.0 for all four variants in this setting and is therefore omitted from Table~\ref{tab:ablation_components}. Random feasible action selection exhibits the largest utility variation and a substantially larger bandwidth-inefficiency term while maintaining delivered quality comparable to the other variants. This result shows that feasibility alone does not make an action efficient. Structured selection is also needed to avoid valid decisions that impose unnecessary network cost.
